# Supplementary material for: Bi-Noising Diffusion: Towards Conditional Diffusion Models with Generative Restoration Priors
Source: arXiv:2212.07352 source file (2022-12-14)
Supplement: Supplementary file 1 [file rain_800_colour_suppl.tex]

\begin{figure}
    \centering
    \setlength{\tabcolsep}{0.5pt}
    {\small
     
    \begin{tabular}{c c c c c c c c c}
    \captionsetup{type=figure, font=scriptsize}
    \raisebox{0.2in}{\rotatebox[origin=t]{90}{Rain}}&
    \includegraphics[width=0.25\linewidth]{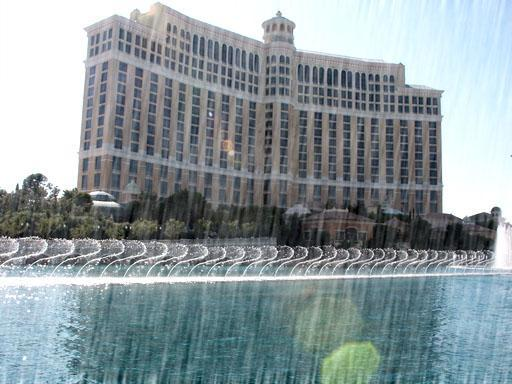}&
    \includegraphics[width=0.25\linewidth]{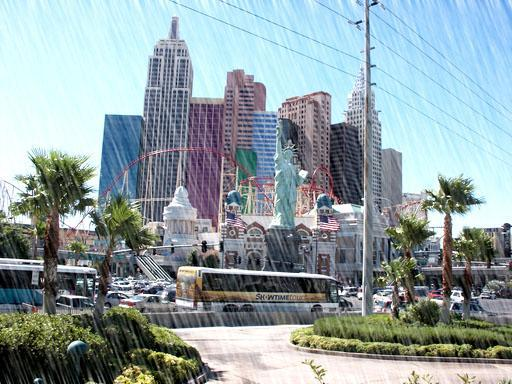}&
    \includegraphics[width=0.25\linewidth]{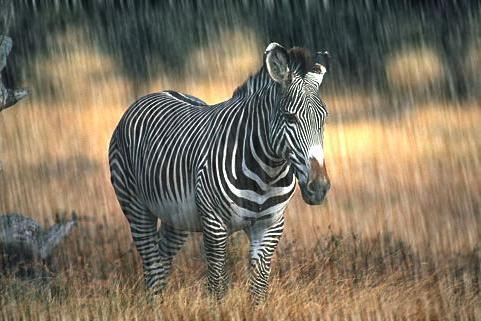}&
    \includegraphics[width=0.25\linewidth]{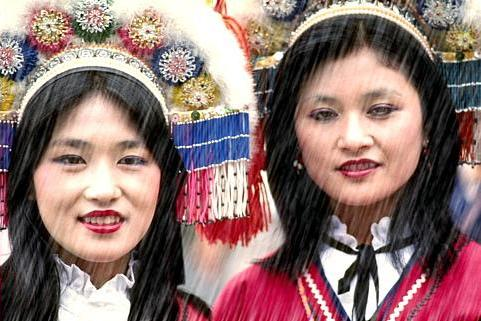}&

    \tabularnewline
    \raisebox{0.2in}{\rotatebox[origin=t]{90}{LDRP\cite{saharia2021image}}}&
    \includegraphics[width=0.25\linewidth]{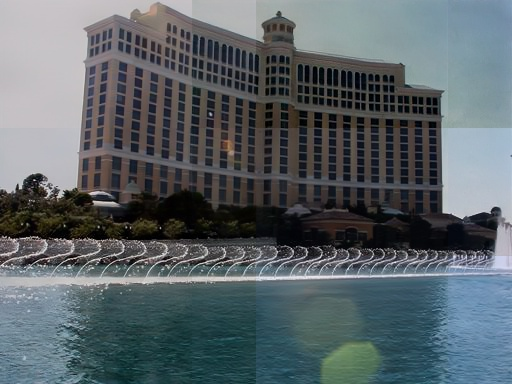}&
    \includegraphics[width=0.25\linewidth]{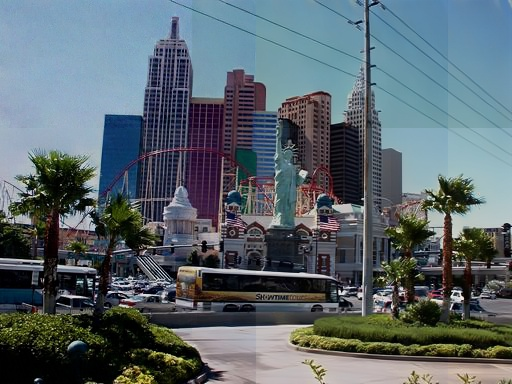}&
    \includegraphics[width=0.25\linewidth]{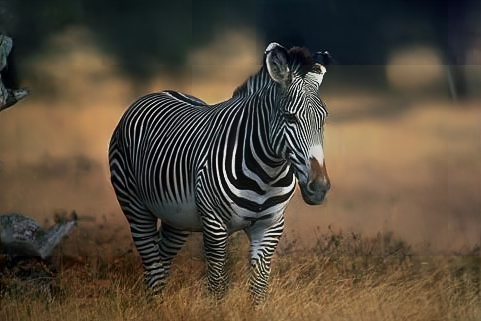}&
    \includegraphics[width=0.25\linewidth]{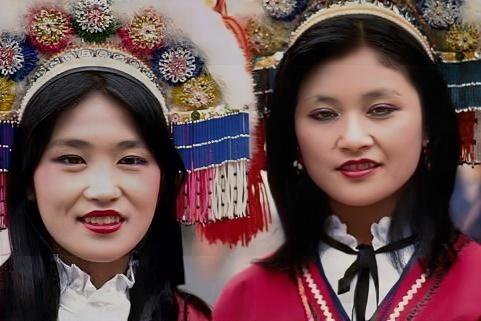}&

    \tabularnewline
    \raisebox{0.2in}{\rotatebox[origin=t]{90}{OURS}}&
    \includegraphics[width=0.25\linewidth]{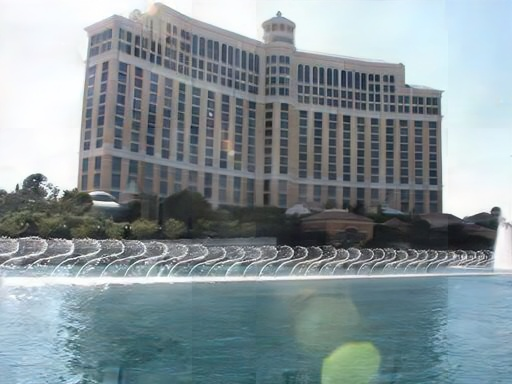}&
    \includegraphics[width=0.25\linewidth]{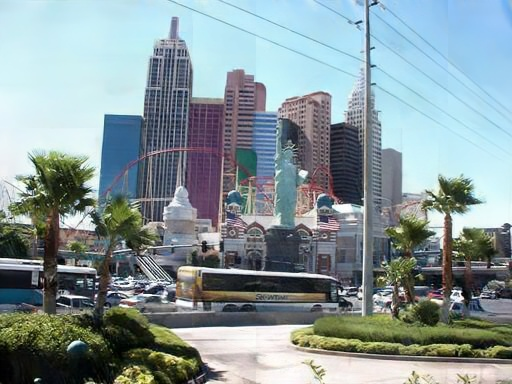}&
    \includegraphics[width=0.25\linewidth]{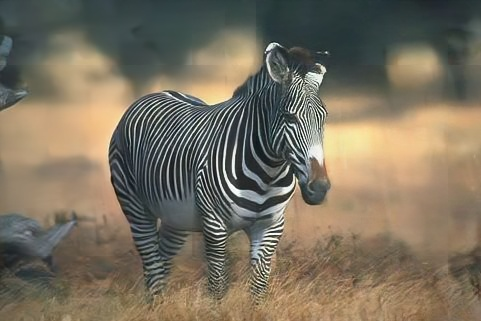}&
    \includegraphics[width=0.25\linewidth]{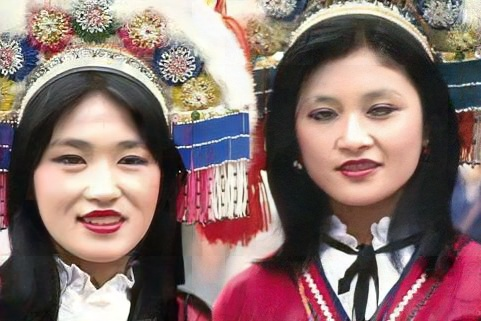}&

    \tabularnewline
    \tabularnewline
    \raisebox{0.2in}{\rotatebox[origin=t]{90}{GT}}&
    \includegraphics[width=0.25\linewidth]{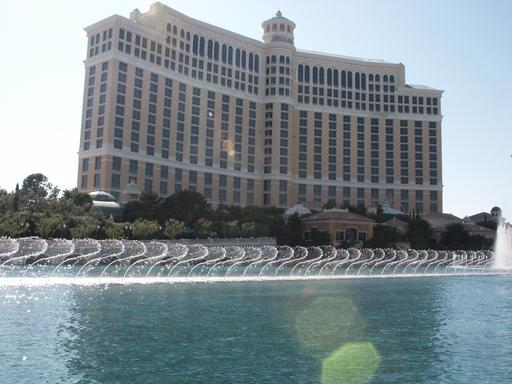}&
    \includegraphics[width=0.25\linewidth]{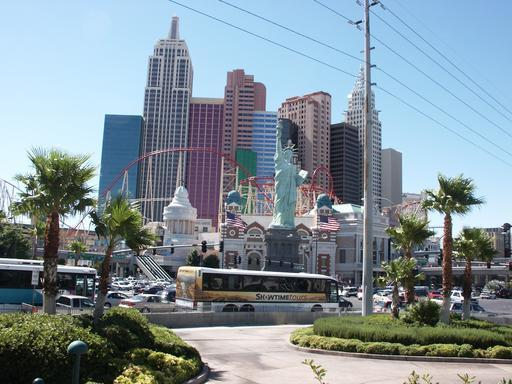}&
    \includegraphics[width=0.25\linewidth]{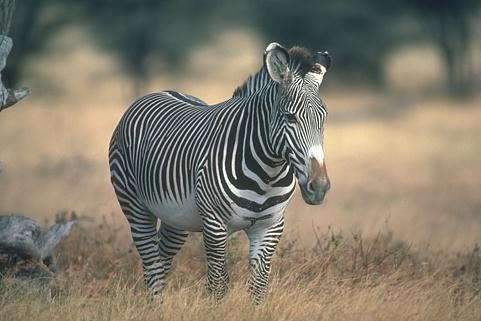}&
    \includegraphics[width=0.25\linewidth]{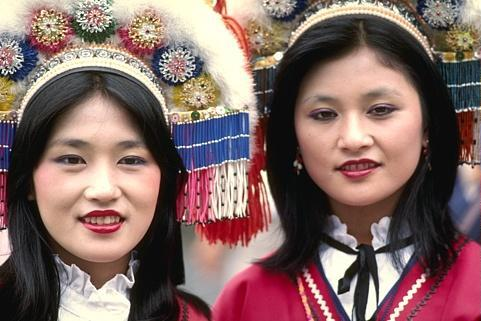}&

\end{tabular}}
\caption{ Visualization of Deraining results on Rain 800 dataset\cite{zhang2019image}. Please note the colour shift happening when trained without the modified losses. (Zoom for better view)}
\label{fig:rain800_supp}
\end{figure}
